# Supplementary material for: Retrieval Augmented Structured Generation: Business Document Information Extraction As Tool Use
Source: arXiv:2405.20245 source file (2024-05-30)
Supplement: Supplementary file 1 [file 7-appendix.tex]

\appendix

\section{Supplementary Material}

\subsection{Ablation Benchmarks}

\begin{table*}[ht]

\centering
\caption{Ablation Benchmark Raw Results for Key-Information Extraction (KIE) with GPT-3.5}
\ifthenelse{\boolean{isaclsubmission}}{}{\rowcolors{1}{}{gray!5}}
\begin{tabular}{cccr}
    \toprule
    1-Shot Retrieval & Supervised Fine-Tuning & Structured Prompting  & F1 Score \\
    \midrule
    \cmark & \cmark & \cmark & \textbf{75.40\%} \\
    \xmark & \cmark & \cmark & \textbf{72.72\%} \\
    \cmark & \cmark & \xmark & \textbf{69.48\%} \\
    \cmark & \xmark & \cmark & \textbf{67.87\%} \\
    \cmark & \xmark & \xmark & \textbf{66.78\%} \\
    \xmark & \cmark & \xmark & 62.40\% \\
    \xmark & \xmark & \cmark & 29.30\%\\
    \xmark & \xmark & \xmark & 26.80\%\\
    \bottomrule
\end{tabular}

\bigskip
\centering
\caption{Ablation Benchmark Raw Results for Key-Information Extraction (KIE) with Hermes 2 Pro}
\begin{tabular}{cccr}
    \toprule
    1-Shot Retrieval & Supervised Fine-Tuning & Structured Prompting  & F1 Score \\
    \midrule
    \cmark & \cmark & \cmark & \textbf{73.41\%} \\
    \cmark & \cmark & \xmark & 68.82\% \\
    \cmark & \xmark & \xmark & 48.42\% \\
    \cmark & \xmark & \cmark & 47.71\% \\
    \xmark & \cmark & \xmark & 29.68\% \\
    \xmark & \cmark & \cmark & 28.13\% \\
    \xmark & \xmark & \cmark & 16.62\%\\
    \xmark & \xmark & \xmark & 16.44\%\\
    \bottomrule
\end{tabular}
\end{table*}

\begin{table*}[ht]
\centering
\caption{Ablation Benchmark Raw Results for Line Items Recognition (LIR) with GPT-3.5}
\begin{tabular}{cccr}
    \toprule
    1-Shot Retrieval & Supervised Fine-Tuning & Structured Prompting  & GLIRM-F1 Score \\
    \midrule
    \cmark & \cmark & \cmark & \textbf{79.81\%} \\
    \xmark & \cmark & \cmark & \textbf{77.52\%} \\
    \cmark & \xmark & \cmark & \textbf{72.12\%} \\
    \cmark & \xmark & \xmark & 58.26\% \\
    \cmark & \cmark & \xmark & 48.72\% \\
    \xmark & \cmark & \xmark & 48.72\% \\
    \xmark  & \xmark & \cmark & 38.25\% \\
    \xmark & \xmark & \xmark & 23.03\% \\
    \bottomrule
\end{tabular}

\bigskip
\centering
\caption{Ablation Benchmark Raw Results for Line Items Recognition (LIR) with Hermes 2 Pro}
\begin{tabular}{cccr}
    \toprule
    1-Shot Retrieval & Supervised Fine-Tuning & Structured Prompting  & GLIRM-F1 Score \\
    \midrule
    \cmark & \cmark & \cmark & 69.44\% \\
    \cmark & \cmark & \xmark & 56.80\% \\
    \cmark & \xmark & \cmark & 55.02\% \\
    \cmark & \xmark & \xmark & 47.35\% \\
    \xmark & \cmark & \cmark & 36.61\% \\
    \xmark & \cmark & \xmark & 11.74\% \\
    \xmark & \xmark & \xmark & 11.02\% \\
    \xmark & \xmark & \cmark & 7.06\% \\
    \bottomrule
\end{tabular}
\end{table*}
